# Supplementary material for: Quantitative mobile gamma-ray spectrometry through Bayesian inference
Source: arXiv:2512.18769 ancillary file (2026-09-04)
Supplement: Supplementary file 1 [file supplementary_materials.pdf]

# Supplementary Information for

## Source quantification by mobile gamma-ray spectrometry systems: A Bayesian approach

David Breitenmoser[1,2,*], Alberto Stabilini[1], Malgorzata Magdalena Kasprzak[1], Sabine Mayer[1]

[1]Department of Radiation Safety and Security, Paul Scherrer Institute (PSI), Forschungsstrasse 111, Villigen PSI, 5232, Switzerland

[2]Department of Nuclear Engineering & Radiological Sciences, University of Michigan, 2355 Bonisteel Blvd., Ann Arbor, MI 48109-2104, United States of America

[*]Lead and contact author: David Breitenmoser (E-Mail: david.breitenmoser@psi.ch, ORCID: 0000-0003-0339-6592)

**The PDF includes:**

Supplementary Figures S1–S7
Supplementary Tables S1–S4
Supplementary References

# Contents

**List of Supplementary Figures** SIII

**List of Supplementary Tables** SIV

**S1 Supplementary Figures** S1

**S2 Supplementary Tables** S8

**Supplementary References** S12

# List of Supplementary Figures

S1 Background measurements . . . S1
S2 Trace and convergence plots for the dataset `Cs_1s` . . . S2
S3 Trace and convergence plots for the dataset `Cs_5s` . . . S3
S4 Trace and convergence plots for the dataset `Cs_5m` . . . S4
S5 Trace and convergence plots for the dataset `Ba_1s` . . . S5
S6 Trace and convergence plots for the dataset `Ba_5s` . . . S6
S7 Trace and convergence plots for the dataset `Ba_5m` . . . S7

# List of Supplementary Tables

S1 Radiation measurement meta-data . . . . . . . . . . S8
S2 Prior distribution summary . . . . . . . . . . S9
S3 Posterior distribution summary for the datasets `Cs_1s`, `Cs_5s`, and `Cs_5m` . . . . . . . . . . S10
S4 Posterior distribution summary for the datasets `Ba_1s`, `Ba_5s`, and `Ba_5m` . . . . . . . . . . S11

# S1 Supplementary Figures

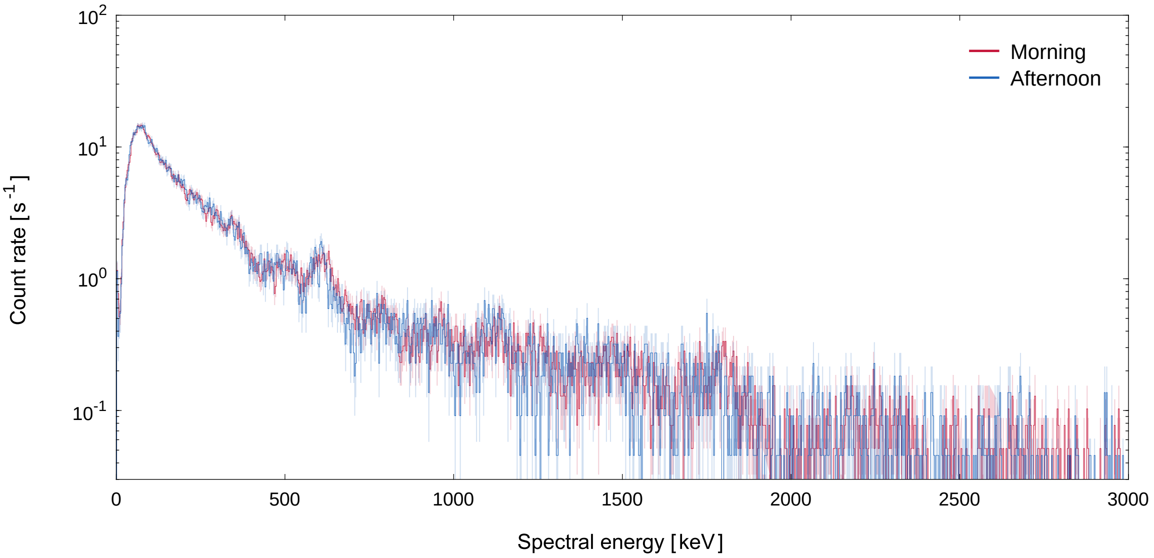


**Figure S1 Background measurements.** Here, we display the measured background pulse-height spectra as a function of the spectral energy with a spectral energy bin width of ~3 keV. The spectra were acquired by the Swiss Airborne Gamma-Ray Spectrometry (SAGRS) system [1] in the morning and afternoon on June 16, 2022 over Lake Thun during the ARM22 validation campaign [2] at orthometric heights equivalent to the ones of the hover flight measurements utilized in the main study, i.e., 659(5) m for the hover flight with the $^{137}_{55}$Cs source (morning) and 659(6) m for the hover flight with the $^{133}_{56}$Ba source (afternoon), respectively. Uncertainties are provided as 1 standard error shaded areas.

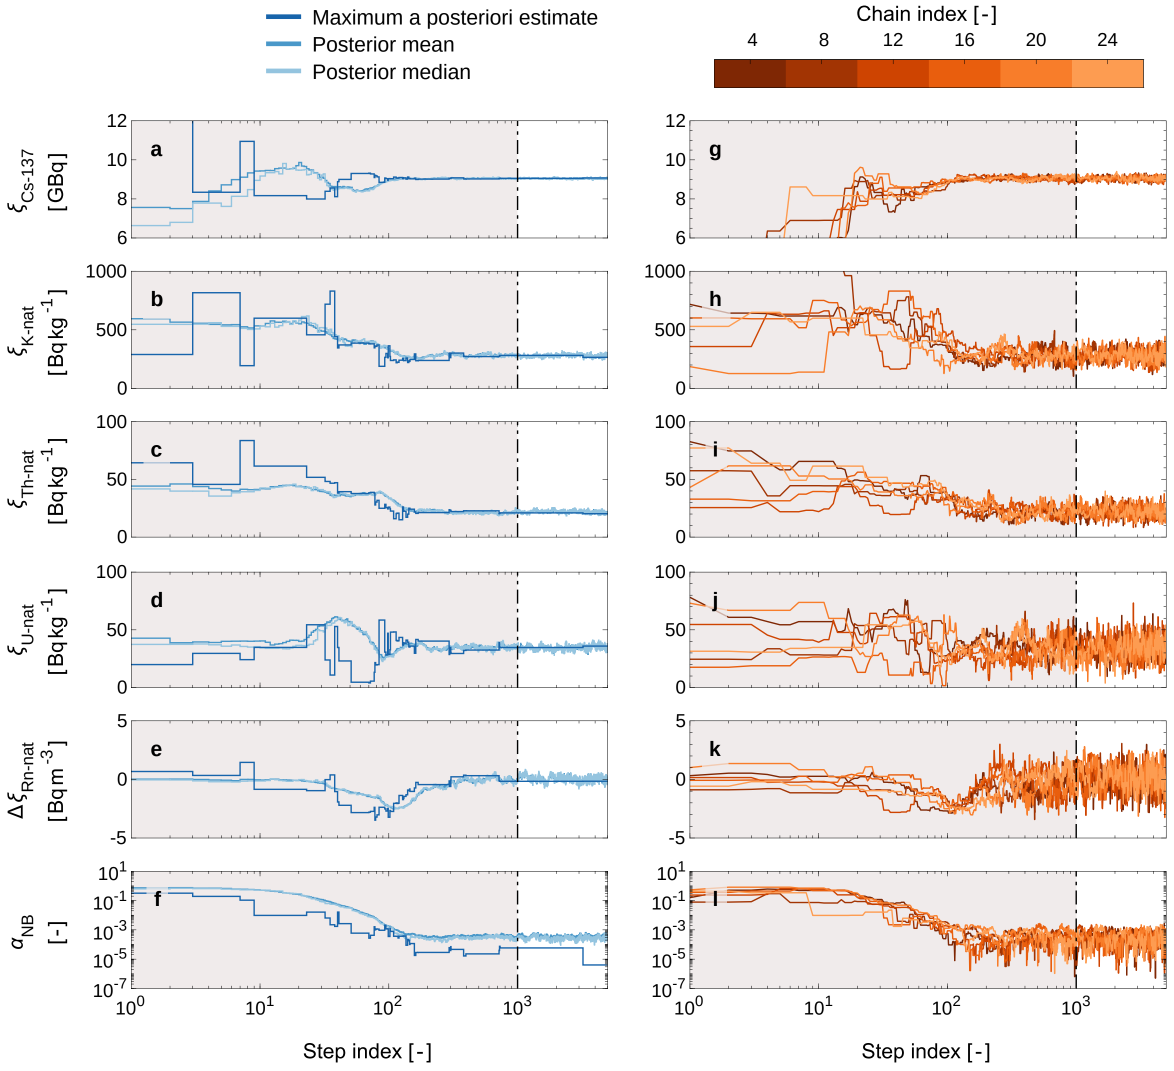


**Figure S2 Trace and convergence plots for the dataset `Cs_1s`.** These graphs present the convergence (**a–f**) and trace (**g–l**) plots for the Markov chain Monte Carlo (MCMC) based Bayesian inversion computations for the dataset `Cs_1s`. The graphs are displayed as a function of the MCMC steps for each model parameter, i.e., the source strength of the sealed $^{137}_{55}$Cs point source ($\xi_{\text{Cs-137}}$), the source strengths of the three natural terrestrial radionuclides $K_{nat}$, $Th_{nat}$ and $U_{nat}$ ($\xi_{\text{K-nat}}$, $\xi_{\text{Th-nat}}$, $\xi_{\text{U-nat}}$), the source strength of the radon source term $\Delta Rn_{nat}$ ($\Delta\xi_{\text{Rn-nat}}$) and the dispersion parameter of the negative binomial distribution ($\alpha_{NB}$). The convergence is shown for the maximum a posteriori estimate, the posterior mean, and the posterior median. The trace plots display a subset of 6 out of the 24 simulated MCMC chains. The burn-in phase is highlighted for all subgraphs as gray-shaded areas with the related threshold marked by the dashed-dotted black line.

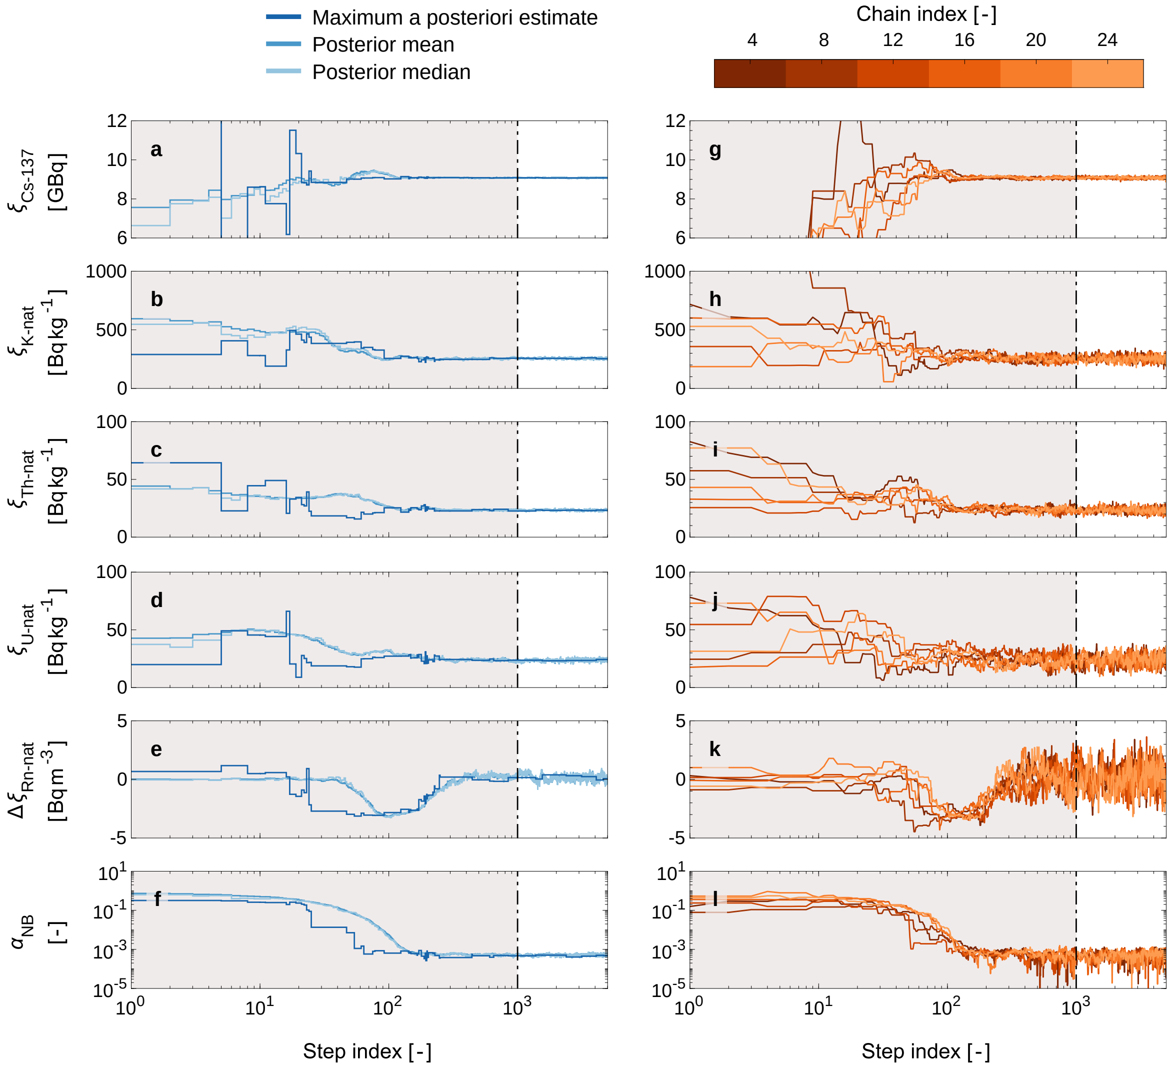


**Figure S3 Trace and convergence plots for the dataset** `Cs_5s`**.** Same as Fig. S2, but using dataset `Cs_5s` instead of dataset `Cs_1s`.

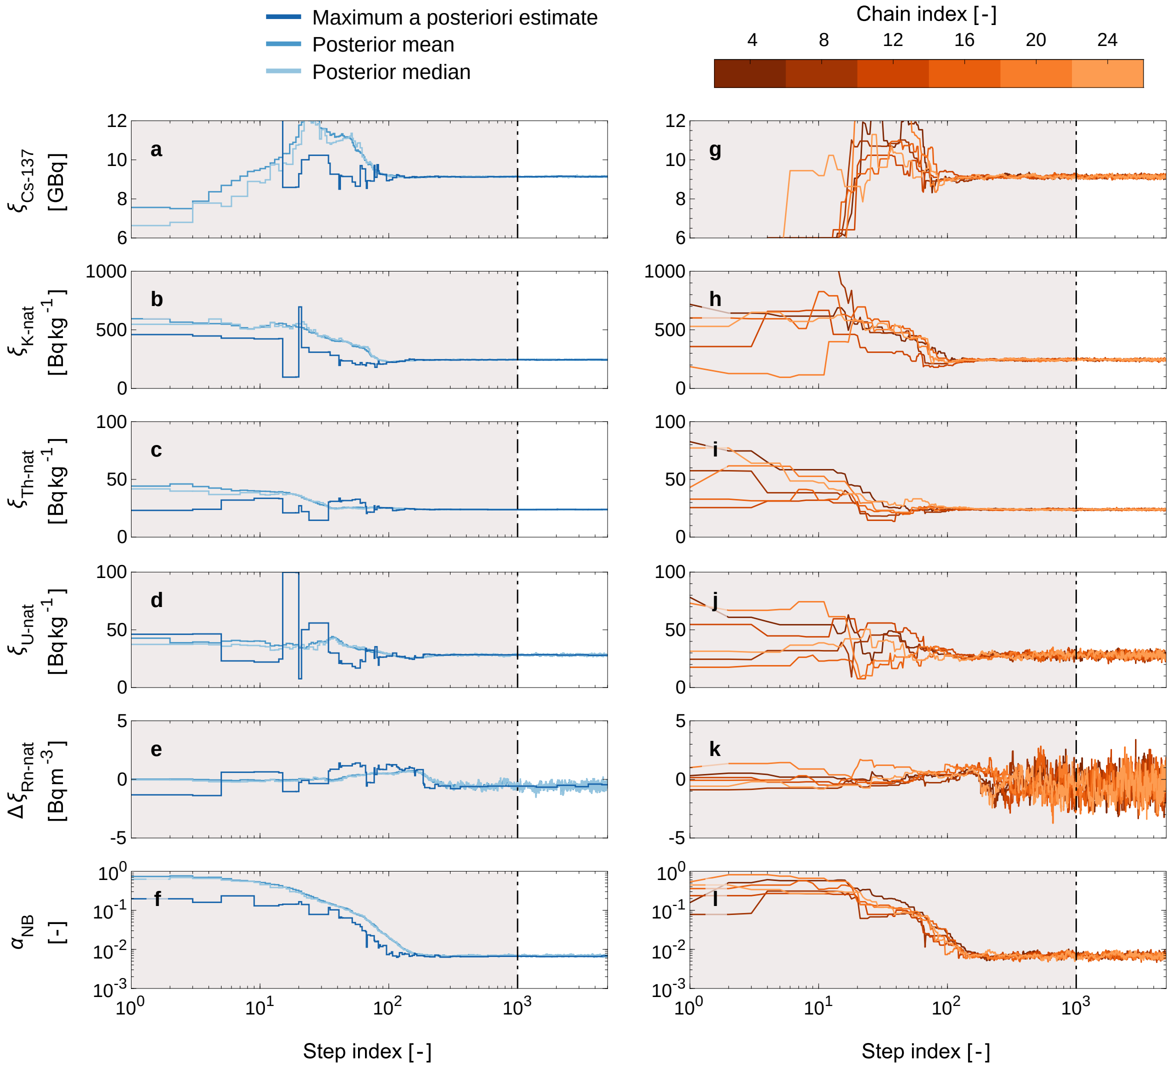


**Figure S4 Trace and convergence plots for the dataset `Cs_5m`.** Same as Fig. S2, but using dataset `Cs_5m` instead of dataset `Cs_1s`.

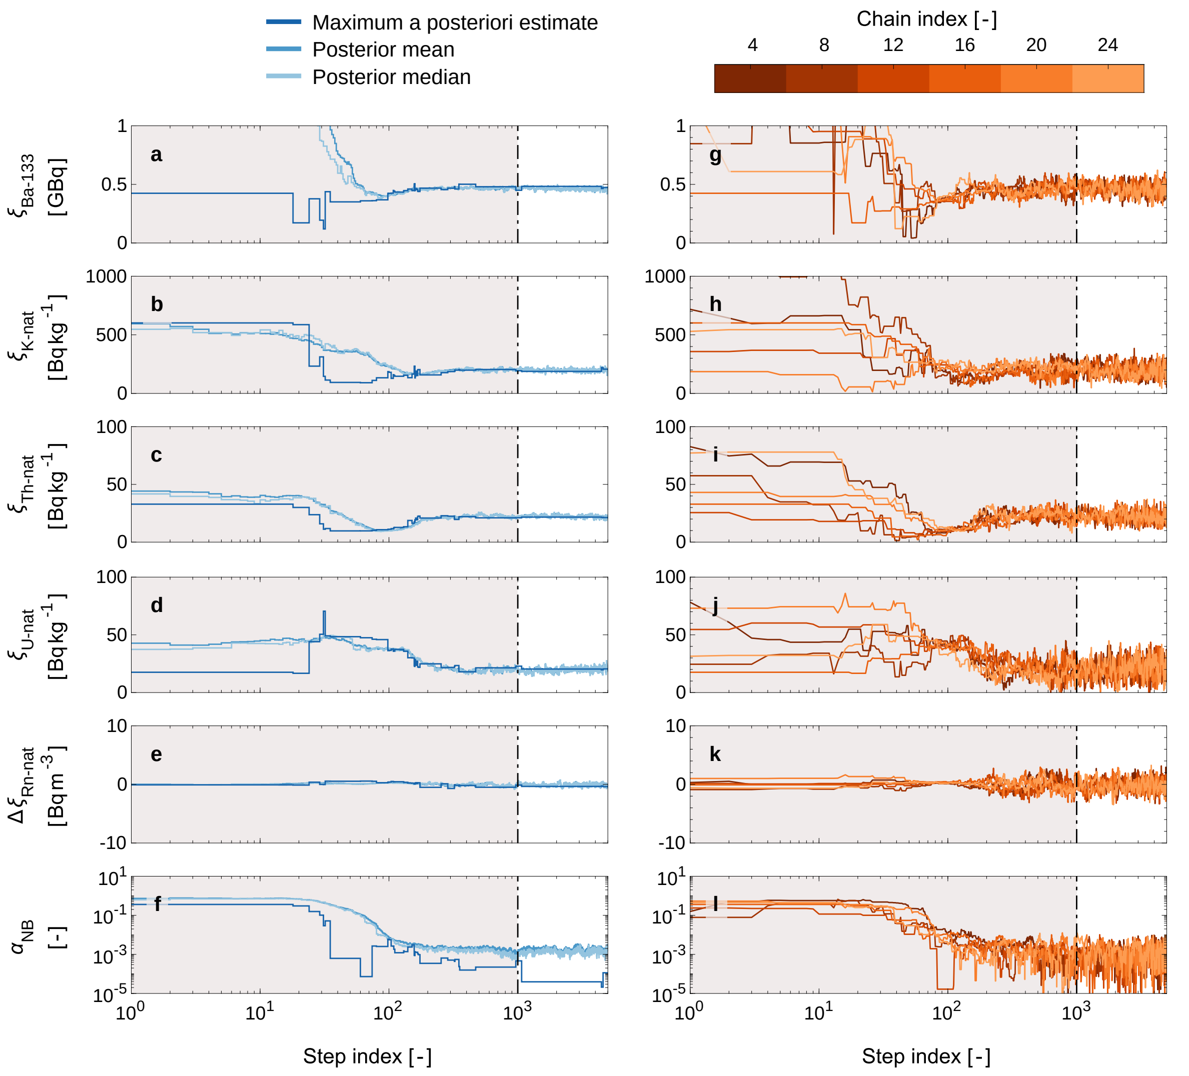


**Figure S5 Trace and convergence plots for the dataset `Ba_1s`.** Same as Fig. S2, but using dataset `Ba_1s` instead of dataset `Cs_1s`.

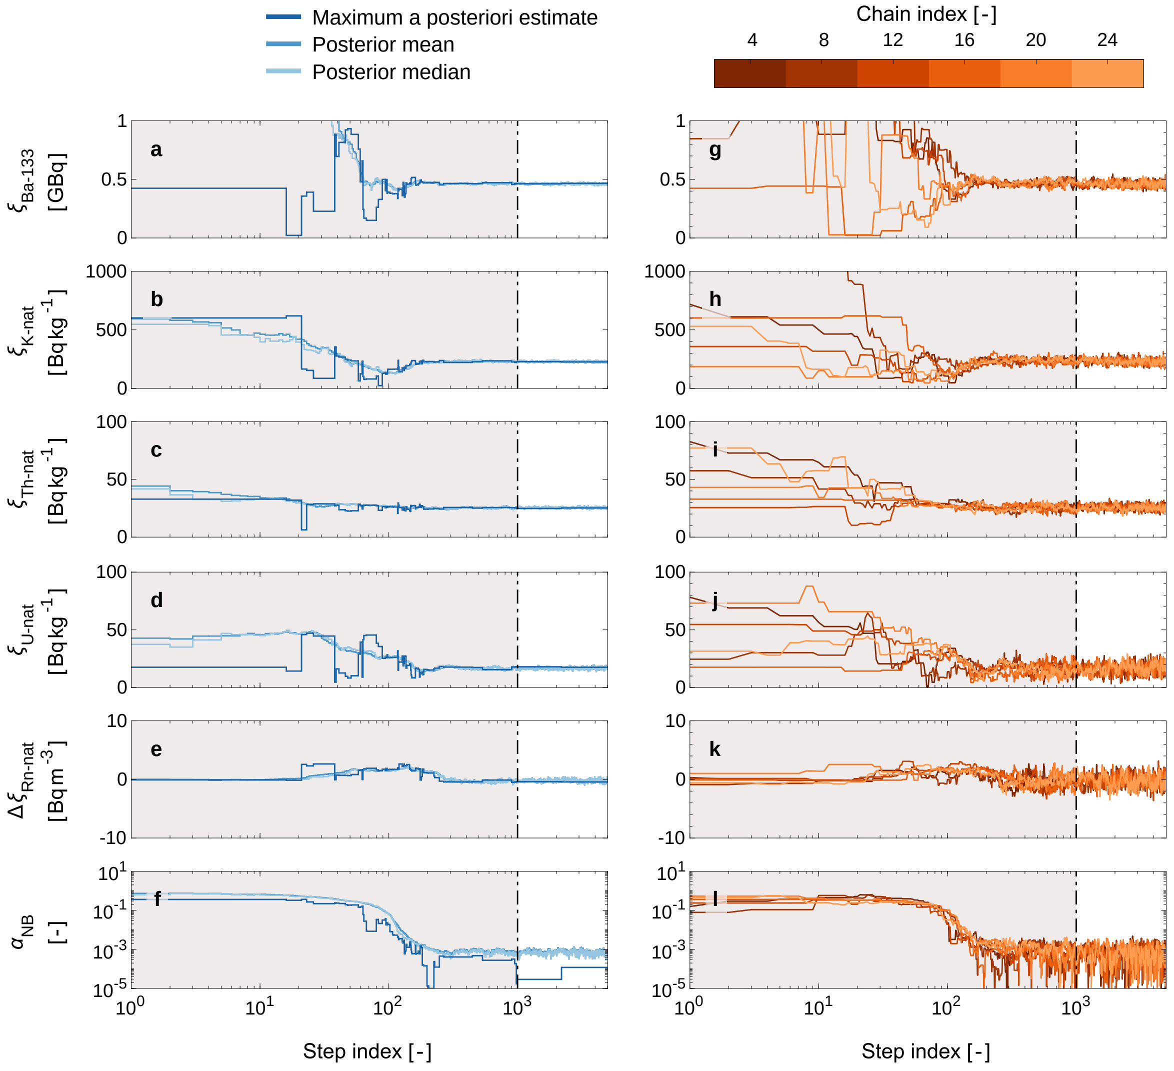


**Figure S6 Trace and convergence plots for the dataset `Ba_5s`.** Same as Fig. S2, but using dataset `Ba_5s` instead of dataset `Cs_1s`.

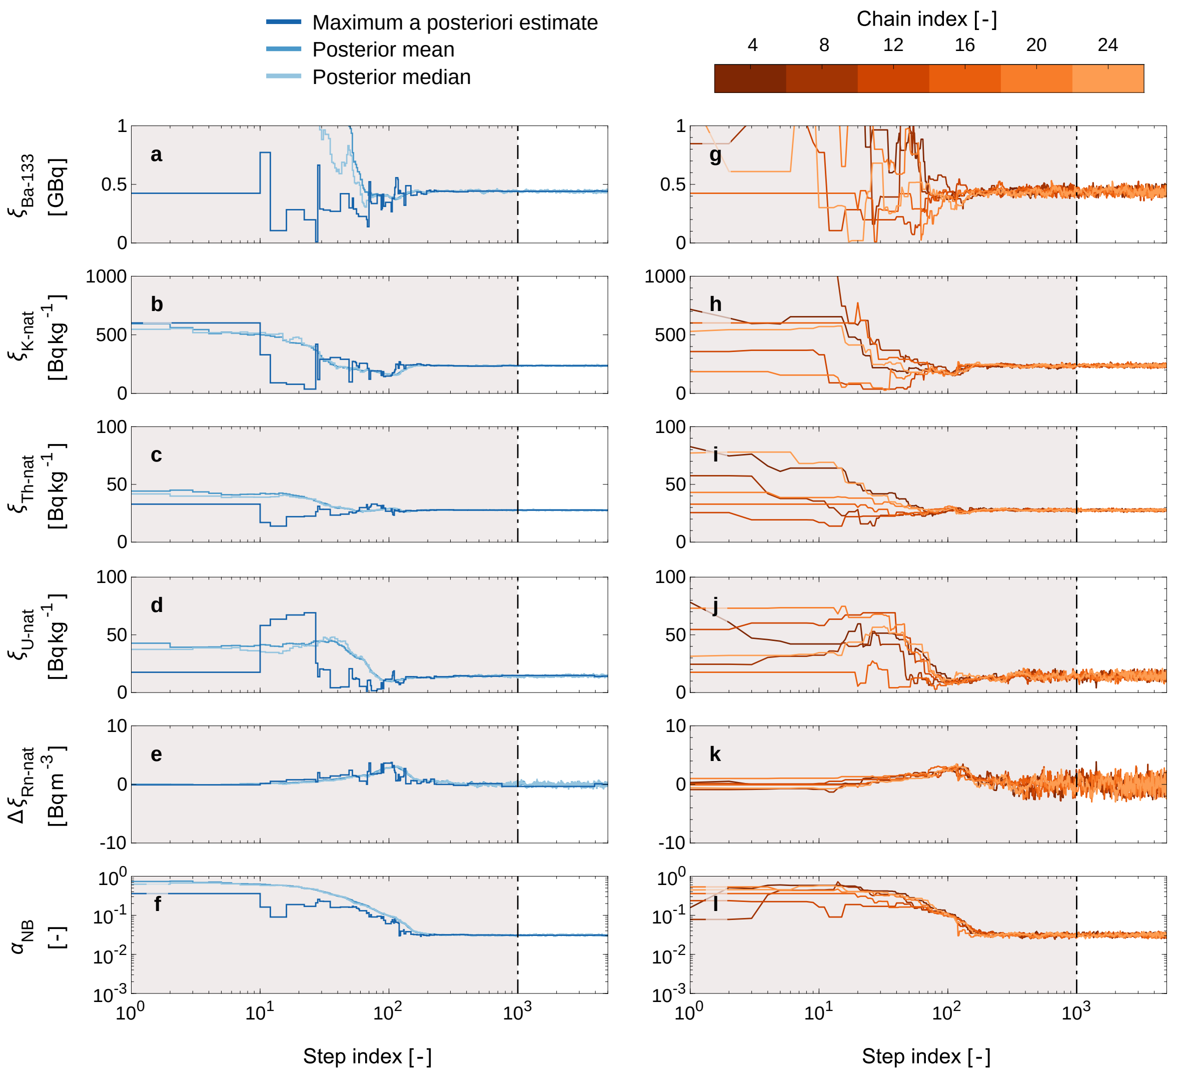


**Figure S7 Trace and convergence plots for the dataset** `Ba_5m`**.** Same as Fig. S2, but using dataset `Ba_5m` instead of dataset `Cs_1s`.

# S2 Supplementary Tables

**Table S1** **Radiation measurement meta-data.** Here, we present an overview of the radiation measurement datasets, highlighting deployed radionuclide sources alongside auxiliary sensor data. Provided uncertainties represent the standard error for the measurement (coverage factor $k = 1$) in least significant figure notation. Please refer to Ref. [1] for a detailed description of the associated radiation measurements and related data postprocessing.

| Identifier | Source⋆ | $\mathscr{A}$• [GBq] | $h_{\mathrm{air}}$∘ [m] | $-\alpha'$† [°] | $\beta'$‡ [°] | $\gamma'$§ [°] | $\varrho_{\mathrm{fuel}}$$ [%] | $T_{\mathrm{air}}$# [°C] | $p_{\mathrm{air}}$•• [hPa] | $\mathrm{RH}_{\mathrm{air}}$∘∘ [%] | $t_{\mathrm{gr}}$†† [s] | $t_{\mathrm{b}}$‡‡ [s] |
|---|---|---|---|---|---|---|---|---|---|---|---|---|
| Ba_1s | $^{133}_{56}$Ba | 0.47(2) | 93(1) | 316(3) | 1(1) | −0.2(1) | 94(2) | 17.4(1) | 953.7(1) | 85.4(1) | 1 | 260 |
| Ba_5s | $^{133}_{56}$Ba | 0.47(2) | 92(1) | 314(3) | −0.33(5) | −1.5(1) | 94(2) | 17.4(1) | 953.7(1) | 85.4(1) | 5 | 260 |
| Ba_5m | $^{133}_{56}$Ba | 0.47(2) | 90.8(1) | 314(3) | −0.34(4) | −1.3(1) | 94(2) | 17.4(1) | 953.7(1) | 85.4(1) | 296 | 260 |
| Cs_1s | $^{137}_{55}$Cs | 9.0(5) | 88(2) | 142(3) | 0.6(1) | −2.6(1) | 57(2) | 26.1(1) | 954.8(1) | 59.6(1) | 1 | 298 |
| Cs_5s | $^{137}_{55}$Cs | 9.0(5) | 91(2) | 142(3) | 0.6(1) | −3.0(1) | 57(2) | 26.1(1) | 954.8(1) | 59.6(1) | 5 | 298 |
| Cs_5m | $^{137}_{55}$Cs | 9.0(5) | 91.6(2) | 142(3) | 0.6(1) | −2.9(1) | 57(2) | 26.1(1) | 954.8(1) | 59.6(1) | 232 | 298 |

⋆ Radionuclide source adopted in the corresponding gross measurement.
• Mean source activity.
∘ Mean ground clearance of the gross measurement determined by the radar altimeter of the AS332M1 helicopter. Note that the data was corrected for the vertical displacement between the radar altimeter, located at the bottom of the tail, and the spectrometer, mounted in the cargo bay (see Ref. [1]).
† Mean negative yaw angle relative to geographic north.
‡ Mean roll angle.
§ Mean pitch angle.
$ Mean fuel volume fraction. For the Monte Carlo simulations, the individual fuel volume fractions of the six tanks were adopted (see Ref. [1]). Here, we report only the average fraction across all tanks.
# Mean air temperature.
•• Mean air pressure.
∘∘ Mean relative humidity.
†† Gross measurement live time (rounded to seconds).
‡‡ Background measurement live time (rounded to seconds).

**Table S2 Prior distribution summary.** This table summarizes the marginal prior distributions adopted for the Bayesian inference in the main study. The marginal prior distributions for the source strengths of the natural terrestrial radionuclides $K_{nat}$, $Th_{nat}$, and $U_{nat}$ were motivated by a study by Bennett[3].

| Variable⋆ | Prior• | Prior parameters | | Truncation | Unit |
|---|---|---|---|---|---|
| $\xi_{\text{Cs-137}}$ | $\mathcal{N}$ | $\mu = 10^9$ | $\sigma = 10^{10}$ | $[0, \infty]$ | Bq |
| $\xi_{\text{Ba-133}}$ | $\mathcal{N}$ | $\mu = 10^9$ | $\sigma = 10^{10}$ | $[0, \infty]$ | Bq |
| $\xi_{\text{K-nat}}$ | $\mathcal{N}$ | $\mu = 350$ | $\sigma = 600$ | $[0, \infty]$ | $\text{Bq kg}^{-1}$ |
| $\xi_{\text{Th-nat}}$ | $\mathcal{N}$ | $\mu = 25$ | $\sigma = 43$ | $[0, \infty]$ | $\text{Bq kg}^{-1}$ |
| $\xi_{\text{U-nat}}$ | $\mathcal{N}$ | $\mu = 25$ | $\sigma = 40$ | $[0, \infty]$ | $\text{Bq kg}^{-1}$ |
| $\Delta\xi_{\text{Rn-nat}}$ | $\mathcal{N}$ | $\mu = 0$ | $\sigma = 1$ | $[-\infty, \infty]$ | $\text{Bq m}^{-3}$ |
| $\alpha_{\text{NB}}$ | $\mathcal{N}$ | $\mu = 0$ | $\sigma = 1$ | $[0, \infty]$ | |

⋆ Model parameters considered in the Bayesian inference, i.e., the source strengths of the sealed $^{137}_{55}Cs$ and $^{133}_{56}Ba$ point sources ($\xi_{\text{Cs-137}}$, $\xi_{\text{Ba-133}}$), the source strengths of the three natural terrestrial radionuclides $K_{nat}$, $Th_{nat}$ and $U_{nat}$ ($\xi_{\text{K-nat}}$, $\xi_{\text{Th-nat}}$, $\xi_{\text{U-nat}}$), the source strength of the radon source term $\Delta Rn_{nat}$ ($\Delta\xi_{\text{Rn-nat}}$) and the dispersion parameter of the negative binomial distribution ($\alpha_{\text{NB}}$).

• With $\mathcal{N}$, we refer to the truncated univariate normal distribution $\mathcal{N}(\mu, \sigma, \theta_l, \theta_u)$ with mean $\mu$, standard deviation $\sigma$ and truncation $\theta \in [\theta_l, \theta_u]$, parametrized by the lower and upper boundary parameters $\theta_l$ and $\theta_u$.

**Table S3 Posterior distribution summary for the datasets `Cs_1s`, `Cs_5s`, and `Cs_5m`.** This table includes posterior point and dispersion estimators for the datasets `Cs_1s`, `Cs_5s`, and `Cs_5m` discussed in the main study. The listed estimators are the maximum a posteriori estimate ($\theta_{MAP}$), the posterior mean ($\theta_{Mean}$), and the posterior median ($\theta_{Median}$) together with the 95 % credible interval and the posterior standard deviation ($\sigma_\theta$). All numerical values displayed are rounded to three significant digits.

| **ID**⋆ | **Variable**• | $\theta_{MAP}$ | $\theta_{Mean}$ | $\theta_{Median}$ | **95 % credible interval**∘ | $\sigma_\theta$ | **Unit** |
|---|---|---|---|---|---|---|---|
| `Cs_1s` | $\xi_{Cs\text{-}137}$ | $9.07 \times 10^{9}$ | $9.05 \times 10^{9}$ | $9.05 \times 10^{9}$ | $[8.85, 9.23] \times 10^{9}$ | $9.65 \times 10^{7}$ | Bq |
| | $\xi_{K\text{-}nat}$ | $2.65 \times 10^{2}$ | $2.81 \times 10^{2}$ | $2.80 \times 10^{2}$ | $[1.87, 3.79] \times 10^{2}$ | $4.90 \times 10^{1}$ | $Bq\,kg^{-1}$ |
| | $\xi_{Th\text{-}nat}$ | $2.03 \times 10^{1}$ | $2.19 \times 10^{1}$ | $2.18 \times 10^{1}$ | $[1.32, 3.13] \times 10^{1}$ | 4.63 | $Bq\,kg^{-1}$ |
| | $\xi_{U\text{-}nat}$ | $3.59 \times 10^{1}$ | $3.47 \times 10^{1}$ | $3.47 \times 10^{1}$ | $[1.79, 5.14] \times 10^{1}$ | 8.53 | $Bq\,kg^{-1}$ |
| | $\Delta\xi_{Rn\text{-}nat}$ | $-1.56 \times 10^{-1}$ | $4.28 \times 10^{-2}$ | $4.16 \times 10^{-2}$ | $[-1.90, 1.97]$ | $9.94 \times 10^{-1}$ | $Bq\,m^{-3}$ |
| | $\alpha_{NB}$ | $4.02 \times 10^{-6}$ | $3.82 \times 10^{-4}$ | $2.78 \times 10^{-4}$ | $[1.02, 134] \times 10^{-5}$ | $3.60 \times 10^{-4}$ | |
| `Cs_5s` | $\xi_{Cs\text{-}137}$ | $9.08 \times 10^{9}$ | $9.08 \times 10^{9}$ | $9.08 \times 10^{9}$ | $[8.98, 9.17] \times 10^{9}$ | $4.87 \times 10^{7}$ | Bq |
| | $\xi_{K\text{-}nat}$ | $2.53 \times 10^{2}$ | $2.56 \times 10^{2}$ | $2.56 \times 10^{2}$ | $[2.11, 3.01] \times 10^{2}$ | $2.28 \times 10^{1}$ | $Bq\,kg^{-1}$ |
| | $\xi_{Th\text{-}nat}$ | $2.33 \times 10^{1}$ | $2.33 \times 10^{1}$ | $2.33 \times 10^{1}$ | $[1.93, 2.78] \times 10^{1}$ | 2.11 | $Bq\,kg^{-1}$ |
| | $\xi_{U\text{-}nat}$ | $2.43 \times 10^{1}$ | $2.37 \times 10^{1}$ | $2.37 \times 10^{1}$ | $[1.51, 3.24] \times 10^{1}$ | 4.41 | $Bq\,kg^{-1}$ |
| | $\Delta\xi_{Rn\text{-}nat}$ | $6.44 \times 10^{-2}$ | $1.36 \times 10^{-1}$ | $1.47 \times 10^{-1}$ | $[-1.79, 2.08]$ | $9.85 \times 10^{-1}$ | $Bq\,m^{-3}$ |
| | $\alpha_{NB}$ | $4.80 \times 10^{-4}$ | $5.35 \times 10^{-4}$ | $5.10 \times 10^{-4}$ | $[1.44, 10.6] \times 10^{-4}$ | $2.33 \times 10^{-4}$ | |
| `Cs_5m` | $\xi_{Cs\text{-}137}$ | $9.15 \times 10^{9}$ | $9.14 \times 10^{9}$ | $9.14 \times 10^{9}$ | $[9.03, 9.26] \times 10^{9}$ | $5.82 \times 10^{7}$ | Bq |
| | $\xi_{K\text{-}nat}$ | $2.44 \times 10^{2}$ | $2.45 \times 10^{2}$ | $2.45 \times 10^{2}$ | $[2.34, 2.55] \times 10^{2}$ | 5.50 | $Bq\,kg^{-1}$ |
| | $\xi_{Th\text{-}nat}$ | $2.39 \times 10^{1}$ | $2.39 \times 10^{1}$ | $2.39 \times 10^{1}$ | $[2.31, 2.47] \times 10^{1}$ | $4.13 \times 10^{-1}$ | $Bq\,kg^{-1}$ |
| | $\xi_{U\text{-}nat}$ | $2.80 \times 10^{1}$ | $2.83 \times 10^{1}$ | $2.83 \times 10^{1}$ | $[2.43, 3.21] \times 10^{1}$ | 2.00 | $Bq\,kg^{-1}$ |
| | $\Delta\xi_{Rn\text{-}nat}$ | $-4.54 \times 10^{-1}$ | $-5.59 \times 10^{-1}$ | $-5.70 \times 10^{-1}$ | $[-2.45, 1.40]$ | $9.81 \times 10^{-1}$ | $Bq\,m^{-3}$ |
| | $\alpha_{NB}$ | $6.82 \times 10^{-3}$ | $6.90 \times 10^{-3}$ | $6.87 \times 10^{-3}$ | $[5.56, 8.45] \times 10^{-3}$ | $7.43 \times 10^{-4}$ | |

⋆ Dataset identifier.
• Model parameters $\theta$ considered in the Bayesian inference, i.e., the source strength of the sealed $^{137}_{55}Cs$ point source ($\xi_{Cs\text{-}137}$), the source strengths of the three natural terrestrial radionuclides $K_{nat}$, $Th_{nat}$, and $U_{nat}$ ($\xi_{K\text{-}nat}$, $\xi_{Th\text{-}nat}$, $\xi_{U\text{-}nat}$), the source strength of the radon source term $\Delta Rn_{nat}$ ($\Delta\xi_{Rn\text{-}nat}$), and the dispersion parameter of the negative binomial distribution ($\alpha_{NB}$).
∘ Central credible interval with a probability mass of 95 %.

**Table S4 Posterior distribution summary for the datasets `Ba_1s`, `Ba_5s`, and `Ba_5m`.** The same as Table S3, but using the datasets `Ba_1s`, `Ba_5s`, and `Ba_5m` instead of the datasets `Cs_1s`, `Cs_5s`, and `Cs_5m`.

| ID⋆ | Variable• | $\theta_{MAP}$ | $\theta_{Mean}$ | $\theta_{Median}$ | 95 % credible interval◦ | $\sigma_\theta$ | Unit |
|---|---|---|---|---|---|---|---|
| `Ba_1s` | $\xi_{Ba\text{-}133}$ | $4.73 \times 10^{8}$ | $4.62 \times 10^{8}$ | $4.63 \times 10^{8}$ | $[3.68, 5.54] \times 10^{8}$ | $4.68 \times 10^{7}$ | Bq |
| | $\xi_{K\text{-}nat}$ | $2.07 \times 10^{2}$ | $1.99 \times 10^{2}$ | $1.98 \times 10^{2}$ | $[1.08, 2.94] \times 10^{2}$ | $4.75 \times 10^{1}$ | $Bq\,kg^{-1}$ |
| | $\xi_{Th\text{-}nat}$ | $2.13 \times 10^{1}$ | $2.23 \times 10^{1}$ | $2.22 \times 10^{1}$ | $[1.43, 3.10] \times 10^{1}$ | 4.25 | $Bq\,kg^{-1}$ |
| | $\xi_{U\text{-}nat}$ | $2.05 \times 10^{1}$ | $2.01 \times 10^{1}$ | $2.00 \times 10^{1}$ | [5.42, 35.6] | 7.70 | $Bq\,kg^{-1}$ |
| | $\Delta\xi_{Rn\text{-}nat}$ | $-3.72 \times 10^{-1}$ | $-7.61 \times 10^{-2}$ | $-6.90 \times 10^{-2}$ | [−2.04, 1.87] | $9.99 \times 10^{-1}$ | $Bq\,m^{-3}$ |
| | $\alpha_{NB}$ | $1.15 \times 10^{-4}$ | $1.93 \times 10^{-3}$ | $1.38 \times 10^{-3}$ | $[4.83, 681] \times 10^{-5}$ | $1.84 \times 10^{-3}$ | |
| `Ba_5s` | $\xi_{Ba\text{-}133}$ | $4.66 \times 10^{8}$ | $4.62 \times 10^{8}$ | $4.63 \times 10^{8}$ | $[4.19, 5.04] \times 10^{8}$ | $2.17 \times 10^{7}$ | Bq |
| | $\xi_{K\text{-}nat}$ | $2.26 \times 10^{2}$ | $2.29 \times 10^{2}$ | $2.29 \times 10^{2}$ | $[1.90, 2.70] \times 10^{2}$ | $2.05 \times 10^{1}$ | $Bq\,kg^{-1}$ |
| | $\xi_{Th\text{-}nat}$ | $2.53 \times 10^{1}$ | $2.55 \times 10^{1}$ | $2.55 \times 10^{1}$ | $[2.15, 2.97] \times 10^{1}$ | 2.13 | $Bq\,kg^{-1}$ |
| | $\xi_{U\text{-}nat}$ | $1.76 \times 10^{1}$ | $1.67 \times 10^{1}$ | $1.68 \times 10^{1}$ | [8.89, 24.3] | 3.92 | $Bq\,kg^{-1}$ |
| | $\Delta\xi_{Rn\text{-}nat}$ | $-4.32 \times 10^{-1}$ | $-2.16 \times 10^{-1}$ | $-2.11 \times 10^{-1}$ | [−2.15, 1.71] | $9.89 \times 10^{-1}$ | $Bq\,m^{-3}$ |
| | $\alpha_{NB}$ | $1.19 \times 10^{-4}$ | $8.00 \times 10^{-4}$ | $6.57 \times 10^{-4}$ | $[3.53, 243] \times 10^{-5}$ | $6.35 \times 10^{-4}$ | |
| `Ba_5m` | $\xi_{Ba\text{-}133}$ | $4.41 \times 10^{8}$ | $4.40 \times 10^{8}$ | $4.40 \times 10^{8}$ | $[3.96, 4.85] \times 10^{8}$ | $2.28 \times 10^{7}$ | Bq |
| | $\xi_{K\text{-}nat}$ | $2.37 \times 10^{2}$ | $2.36 \times 10^{2}$ | $2.36 \times 10^{2}$ | $[2.21, 2.53] \times 10^{2}$ | 8.29 | $Bq\,kg^{-1}$ |
| | $\xi_{Th\text{-}nat}$ | $2.75 \times 10^{1}$ | $2.77 \times 10^{1}$ | $2.77 \times 10^{1}$ | $[2.66, 2.88] \times 10^{1}$ | $5.74 \times 10^{-1}$ | $Bq\,kg^{-1}$ |
| | $\xi_{U\text{-}nat}$ | $1.42 \times 10^{1}$ | $1.44 \times 10^{1}$ | $1.44 \times 10^{1}$ | $[1.03, 1.85] \times 10^{1}$ | 2.13 | $Bq\,kg^{-1}$ |
| | $\Delta\xi_{Rn\text{-}nat}$ | $3.58 \times 10^{-4}$ | $-3.37 \times 10^{-2}$ | $-3.76 \times 10^{-2}$ | [−2.95, 1.85] | $9.73 \times 10^{-1}$ | $Bq\,m^{-3}$ |
| | $\alpha_{NB}$ | $3.06 \times 10^{-2}$ | $3.13 \times 10^{-2}$ | $3.12 \times 10^{-2}$ | $[2.69, 3.61] \times 10^{-2}$ | $2.34 \times 10^{-3}$ | |

⋆ Dataset identifier.

• Model parameters $\theta$ considered in the Bayesian inference, i.e., the source strength of the sealed $^{133}_{56}$Ba point source ($\xi_{Ba\text{-}133}$), the source strengths of the three natural terrestrial radionuclides $K_{nat}$, $Th_{nat}$, and $U_{nat}$ ($\xi_{K\text{-}nat}$, $\xi_{Th\text{-}nat}$, $\xi_{U\text{-}nat}$), the source strength of the radon source term $\Delta Rn_{nat}$ ($\Delta\xi_{Rn\text{-}nat}$), and the dispersion parameter of the negative binomial distribution ($\alpha_{NB}$).

◦ Central credible interval with a probability mass of 95 %.

# Supplementary References


1. Breitenmoser, D., Stabilini, A., Kasprzak, M. M. & Mayer, S. Development and Validation of a High-Fidelity Full-Spectrum Monte Carlo Model for the Swiss Airborne Gamma-Ray Spectrometry System. *Nuclear Instruments and Methods in Physics Research Section A: Accelerators, Spectrometers, Detectors and Associated Equipment* **1077,** 170512. doi:10.1016/j.nima.2025.170512. arXiv: 2502.02102 (Aug. 1, 2025).
2. Butterweck, G. *et al. Aeroradiometric Measurements in the Framework of the Swiss Exercise ARM22* (Paul Scherrer Institut (PSI), Villigen PSI, Switzerland, 2023). doi:10.55402/psi:51194.
3. Bennett, B. G. *Natural Background Radiation Exposures World-Wide* in *Int. Conf. High Levels Nat. Radiat.* (eds Sohrabi, M., Ahmed, J. U. & Durrani, S. A.) (International Atomic Energy Agency, Ramsar, 1993), 17–28.
